# Supplementary material for: Direct probe of ferromagnetic proximity effect at the interface in Fe/SnTe heterostructure by polarized neutron reflectometry
Source: arXiv:1910.10540 source file (2019-11-20)
Supplement: Supplementary file 1 [file supporting_information_v5.pdf]

**Supporting information**

# Direct probe of the ferromagnetic proximity effect at the interface of SnTe/Fe heterostructure by polarized neutron reflectometry

Ryota Akiyama,*,† Ryo Ishikawa,‡,‖ Kazuhiro Akutsu,¶ Ryosuke Nakanishi,† Yuta Tomohiro,‡ Kazumi Watanabe,† Kazuki Iida,¶ Masanori Mitome,§ Shuji Hasegawa,† and Shinji Kuroda‡

*†Department of physics, The University of Tokyo, 7-3-1 Hongo, Bunkyo-ku, Tokyo, Japan*
*‡Institute of Materials, University of Tsukuba, 1-1-1 Tennoudai, Tsukuba, Ibaraki, Japan*
*¶Neutron Science and Technology Center, Comprehensive Research Organization for Science and Society (CROSS), 162-1 Shirakata, Tokai, Ibaraki, Japan*
*§Advanced Materials and Nanomaterials Laboratories, National Institute for Materials Science (NIMS), Namiki 1-1, Tsukuba, Ibaraki, Japan*
*‖Current address: Future technology research laboratory, ULVAC, inc., 2-1 Yamadaoka, Suita, Osaka, Japan*

E-mail: akiyama@surface.phys.s.u-tokyo.ac.jp

## Fitting results

In this study, the XRR and PNR measurements were analyzed by the Motofit program. In the fitting of XRR, the structure was assumed to be $Fe_3O_4$/Fe/SnTe. The fitting parameters are SLD and thickness. The resultant fitting parameters of Fig. S1 are listed in table S1.

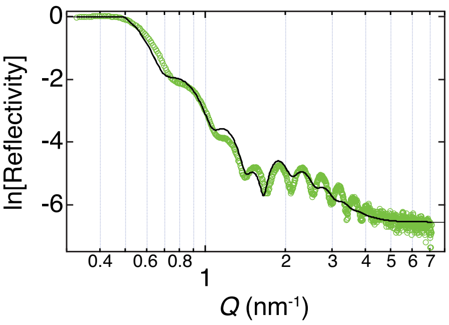


Fig. S1 The $Q$ dependence of reflectivity in XRR .

| | Thickness (nm) | SLD ($10^{-3}$nm$^{-2}$) | Roughness (nm) |
|---|---|---|---|
| $Fe_3O_4$ | 2.30 | 4.09 | 1.05 |
| Fe | 12.40 | 5.60 | 0.35 |
| SnTe | Infinity | 4.90 | 0.69 |

Table S1 The fitting parameters estimated by XRR.

The PNR measurements under 10 kOe at 2.4 K, 150 K and 300 K are displayed in Figs. S2, S3, and S4, respectively. To reveal the ferromagnetic proximity effect from the Fe layer to the SnTe layer, the structure was assumed to be $Fe_3O_4$/Fe/proximity layer/SnTe/CdTe. The estimated fitting parameters are shown in Table S2, S3, and S4, respectively. The red and blue curves represent fitting curves of $R^+$ and $R^-$ reflectivity, respectively.

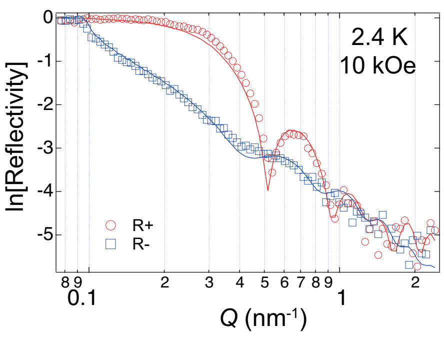


Fig. S2 The $Q$ dependence of reflectivity in PNR at 2.4 K under 10 kOe.

| | Thickness (nm) | SLD ($10^{-4}$ nm$^{-2}$) $R^+/R^-$ | Roughness (nm) |
|---|---|---|---|
| $Fe_3O_4$ | 2.45 | 6.73/5.56 | 0.4 |
| Fe | 12.49 | 13/3.05 | 0.4 |
| Proximity layer | 2.31 | 3.85/1.66 | 0.5 |
| SnTe | 410.00 | 1.89/1.89 | 0.5 |
| CdTe | Infinity | 1.54/1.54 | 0.5 |

Table S2 The fitting parameters estimated by PNR at 2.4 K under 10 kOe.

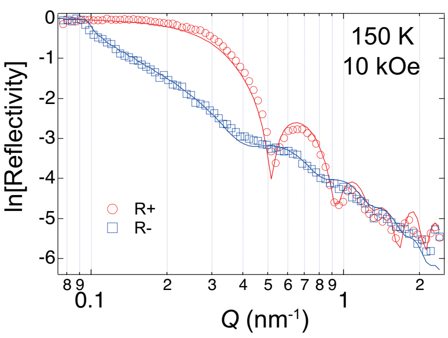


Fig. S3 The $Q$ dependence of reflectivity in PNR at 150 K under 10 kOe.

| | Thickness (nm) | SLD ($10^{-4}$ nm$^{-2}$) $R^+/R^-$ | Roughness (nm) |
|---|---|---|---|
| $Fe_3O_4$ | 2.45 | 6.63/5.46 | 0.4 |
| Fe | 12.49 | 13/3.05 | 0.5 |
| Proximity layer | 2.31 | 3.85/2.03 | 0.5 |
| SnTe | 410.00 | 1.89/1.89 | 0.3 |
| CdTe | Infinity | 1.54/1.54 | 0.5 |

Table S3 The fitting parameters estimated by PNR at 150 K under 10 kOe.

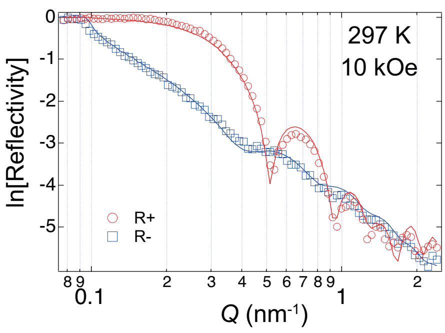


Fig. S4 The $Q$ dependence of reflectivity in PNR at 297 K under 10 kOe.

| | Thickness (nm) | SLD ($10^{-4}$ nm$^{-2}$) $R^+/R^-$ | Roughness (nm) |
|---|---|---|---|
| $Fe_3O_4$ | 2.45 | 6.6/5.3 | 0.4 |
| Fe | 12.49 | 13/3.05 | 0.5 |
| Proximity layer | 2.31 | 3.6925/2.06 | 0.7 |
| SnTe | 410.00 | 1.89/1.89 | 0.2 |
| CdTe | Infinity | 1.54/1.54 | 0.5 |

Table S4 The fitting parameters estimated by PNR at 297 K under 10 kOe.

The differences of magnetization which mean the interfacial magnetization in Fig. S5 (Fig. 5) were fitted by two Gaussian functions. The resultant fitting parameters, magnitude, position, and the full width at half maximum (FWHM) are displayed in Fig. S6 as the temperature dependences.

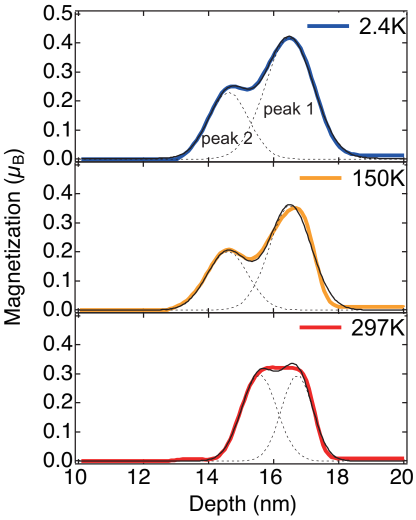


Fig. S5 Extracted depth profiles of the interface magnetizations at 2.4 K, 150 K, and 297 K by subtracting SLD of XRR from MSLD after normalization (blue, orange, and red, respectively).

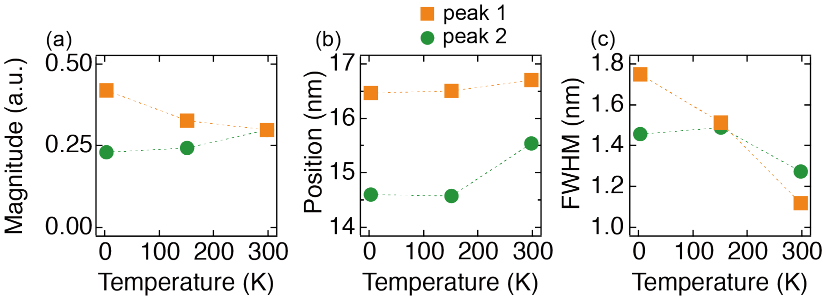


Fig. S6 The temperature dependences of magnitude, position, and FWHM of the two gaussians represented by peak 1 and 2 in Fig. S5.
